# Supplementary material for: Human Activity Recognition Based on Wearable Sensor Data: A Standardization of the State-of-the-Art
Source: arXiv:1806.05226 source file (2019-02-01)
Supplement: Supplementary file 1 [file Appendix.tex]

\section{Appendix}\label{sec::appendix}
\begin{figure*}[!htb]
	\centering
	\subfigure[State-of-the-art on LOSO protocol] {\includegraphics[scale=0.65]{Figures/state_of_the_art.pdf}} 
	\subfigure[State-of-the-art on LOTO protocol] {\includegraphics[scale=0.65]{Figures/state_of_the_art.pdf}}
	
	\subfigure[State-of-the-art on \todo{X} protocol] {\includegraphics[scale=0.65]{Figures/state_of_the_art.pdf}}
	\subfigure[State-of-the-art on \todo{X} protocol] {\includegraphics[scale=0.65]{Figures/state_of_the_art.pdf}}
	\caption{tete}
	\label{fig:state_of_the_art_recall}
\end{figure*}
\begin{table}[]
\centering
\caption{My caption}
\label{my-label}
\begin{tabular}{|c|c|c|c|}
\hline
Method & Top1 & Top2 & Top3 \\ \hline
Kwapisz et al.~\cite{Kwapisz:2010} &  &  &  \\ \hline
Catal et al.~\cite{Catal:2015} &  &  &  \\ \hline
Kim et al.~\cite{Kim:2012} &  &  &  \\ \hline
Kim et al.~\cite{Kim:2013} &  &  &  \\ \hline
Chen and Xue~\cite{ChenChen:2015} & $3$ & $4$ & $5$ \\ \hline
Jiang and Yin~\cite{Jiang:2015} & $0$ & $2$ & $4$ \\ \hline
Ha et al.~\cite{Ha:2015} & $0$ & $0$ & $1$ \\ \hline
Ha and Choi~\cite{Ha:2016} & $0$ & $0$ & $1$ \\ \hline
\end{tabular}
\end{table}
\begin{figure*}[!htb]
	\centering
	\subfigure[State-of-the-art on LOSO protocol] {\includegraphics[scale=0.65]{Figures/state_of_the_art.pdf}} 
	\subfigure[State-of-the-art on LOTO protocol] {\includegraphics[scale=0.65]{Figures/state_of_the_art.pdf}}
	
	\subfigure[State-of-the-art on \todo{X} protocol] {\includegraphics[scale=0.65]{Figures/state_of_the_art.pdf}}
	\subfigure[State-of-the-art on \todo{X} protocol] {\includegraphics[scale=0.65]{Figures/state_of_the_art.pdf}}
	\caption{tete}
	\label{fig:state_of_the_art_acc}
\end{figure*}
\begin{table}[]
\centering
\caption{My caption}
\label{my-label}
\begin{tabular}{|c|c|c|c|}
\hline
Method & Top1 & Top2 & Top3 \\ \hline
Kwapisz et al.~\cite{Kwapisz:2010} &  &  &  \\ \hline
Catal et al.~\cite{Catal:2015} &  &  &  \\ \hline
Kim et al.~\cite{Kim:2012} &  &  &  \\ \hline
Kim et al.~\cite{Kim:2013} &  &  &  \\ \hline
Chen and Xue~\cite{ChenChen:2015} & $3$ & $4$ & $5$ \\ \hline
Jiang and Yin~\cite{Jiang:2015} & $0$ & $2$ & $4$ \\ \hline
Ha et al.~\cite{Ha:2015} & $0$ & $0$ & $1$ \\ \hline
Ha and Choi~\cite{Ha:2016} & $0$ & $0$ & $1$ \\ \hline
\end{tabular}
\end{table}
